# Supplementary material for: Environmental dependence of X-ray and optical properties of galaxy clusters
Source: arXiv:2010.12671 source file (2020-10-23)
Supplement: Supplementary file 1 [file appendix_richnessbias.tex]

\section{Richness bias}
\label{richnesscalc}

We want to investigate possible richness calculation biases of our algorithms between clusters in voids and outside voids. A bias in the richness calculation would mean that the difference in the richness estimation between the two populations is an artefact of the richness estimator algorithm.

For the XCS DR2--SDSS and GMPhoRCC cluster catalogues, the same algorithm, GMPhoRCC, has been used to calculate the richness inside the $R_{200}$ cluster radius. The richness estimation is made by simply counting the numbers of galaxies within a cone with an aperture of $1-4$ arcminutes (depending on the cluster's angular size) and subtracting the number of galaxies in the background in the same aperture. In order to see whether the fact that a cluster resides in a void significantly affects the richness estimation, we can assume a cluster inside a void, like the one in Figure~\ref{fig:clvol}, where the cluster centre is the closest void boundary to us, in order to study the maximum effect. The cluster cone can extend behind the void, depending on the cluster aperture used by GMPhoRCC and the void size. If the error of the background number of galaxies of clusters outside voids, $N_{b,out}$, is larger than the fraction of background galaxies in the part of the cluster cone inside the void, $N_{b,void}$ to all the background galaxies in the cluster cone of clusters inside voids, $N_{b,all}$, then the richness estimation of the clusters inside voids is not significantly biased with respect to that of the clusters outside voids:
\begin{equation}
    Err(N_{b,out}) > \frac{N_{b,void}}{N_{b,all}}= \frac{V_{void}}{V_{all}} \times  \frac{n_{void}}{n_{all}}
	\label{eq:condition}
\end{equation}
where $N$ is the number of background galaxies, $V$ is the volume of the cone, $n$ is the density of the background galaxies and the pointers ``void'', ``out'' and ``all'' show the property is computed inside the voids, outside the voids or both inside and outside of voids respectively. Equation~(\ref{eq:condition}) says that the ratio of galaxies in the part of the cone inside the void to the galaxies in all the cone is equal to the fraction of the volume of the cone inside the void to its total volume times the fraction of the number density in the part of the cone inside the void to the total number density in the cone. 

\begin{figure}
	\centering
	\includegraphics[width=\columnwidth]{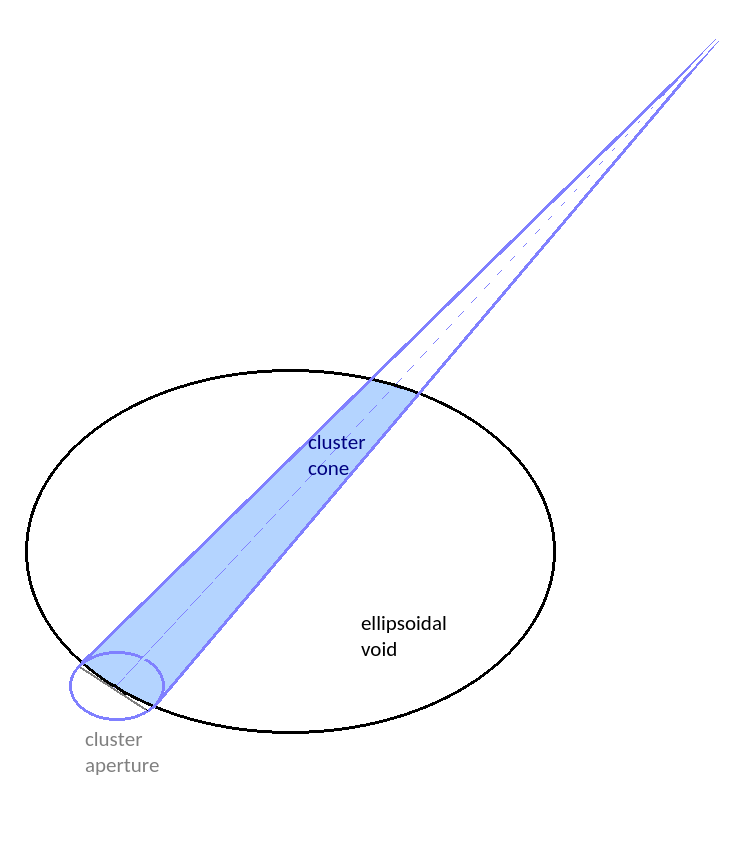}
	\caption{A cluster inside an ellipsoidal void and the cluster cone (in blue) where the GMPhoRCC richness is calculated.}
	\label{fig:clvol}
\end{figure}

The values of $V_{void}/V_{all}$ are calculated by using the void ellipsoidal shapes in LOWZ and CMASS catalogues to find the volume of the cluster cone inside the void and by using the GMPhoRCC aperture to find the total volume of the cluster cone. We calculate the median value of $V_{void}/V_{all}$, which corresponds to the median of the void volumes in the catalogue, the median of the void redshifts and a GMPhoRCC cluster aperture of 2.5 arcminutes. We also calculate the maximum values of $V_{void}/V_{all}$, which correspond to the maximum void volume in the catalogue, the lowest void redshift (the lower redshift the larger fraction of the cone is inside a void so the larger the effect) and a GMPhoRCC cluster aperture of 4 arcminutes. The values for $n_{void}/n_{all}$ are the medians of the density contrast values of the voids as defined in \citet{nadbossvoids} for LOWZ and CMASS. The results for the right hand side of equation~(\ref{eq:condition}) are shown in Table~\ref{tab:volumes}. We compare the last column with the values of the median (and median absolute deviation) error of the background number of galaxies in the XCS DR2--SDSS catalogue, which is 0.3098 (with median absolute deviation 0.2159) and in the GMPhoRCC catalogue, which is 0.1443 (with median absolute deviation 0.1184). These values confirm that equation~(\ref{eq:condition}) holds, which means that the difference found between the richness distributions of clusters in voids and outside voids in the two cluster catalogues is not an artefact of the algorithm that used to calculate the cluster richness.

\begin{table}
	\centering
	\caption{The median (maximum value) of the $V_{void}/V_{all}$, $n_{void}/n_{all}$ and their product (last column) which are the right hand side of the equation~(\ref{eq:condition}).}
	\label{tab:volumes}
	\begin{tabular}{rccc}
		\toprule
		 & $V_{void}/V_{all}$ & $n_{void}/n_{all}$ & Product\\
		\midrule
		LOWZ voids & 0.1112 (0.1119) & 0.2544 & 0.0283\\
		CMASS voids & 0.0766 (0.1322) & 0.2722 & 0.0209\\
	 \bottomrule
	\end{tabular}
\end{table}
